# Supplementary material for: High-Temperature Activation of Single-Photon Emitters in monolayer WS2
Source: arXiv:2512.16579 source file (2025-12-18)
Supplement: Supplementary file 1 [file SI_v2_GJ.pdf]

# High-Temperature Activation of Single-Photon Emitters in monolayer $WS_2$

G. Lee[1], A. Borel[1], T. Taniguchi[2], K. Watanabe[3], F. Sirotti[1], and F. Cadiz[1]

[1]Laboratoire de Physique de la Matière Condensée, CNRS, Ecole polytechnique, Institut Polytechnique de Paris, 91120 Palaiseau, France
[2]Research Center for Materials Nanoarchitectonics, National Institute for Materials Science, 1-1 Namiki, Tsukuba 305-0044, Japan
[3]Research Center for Electronic and Optical Materials, National Institute for Materials Science, 1-1 Namiki, Tsukuba 305-0044, Japan

*Email: fabian.cadiz@polytechnique.edu

## Supporting Information

### Raman features and thermal dissociation of monolayer $WS_2$

Raman spectroscopy was performed on a pre-calibrated micro-membrane (based on its blackbody radiation). The laser source was a 514.5 nm cw laser, spectrally cleaned by a reflective volume Bragg bandpass filter. The scattered light was filtered by two Notch filters centered at the laser wavelength. Figure S1 shows the evolution of the Raman spectra as a function of temperature from 25 °C to 1000 °C under vacuum conditions ($10^{-3}$ mbar). Both the $E_{2g}$ (in-plane vibrational mode) and $A_{1g}$ (out-of-plane vibrational mode) peaks are observed in the Stokes region. With increasing temperature, the Raman peak intensities gradually decrease and eventually vanish at 1000 °C (1273 K), indicating that the $WS_2$ monolayer undergoes thermal dissociation around this temperature. These results indicate that annealing can be safely performed at temperatures below 1000 °C.

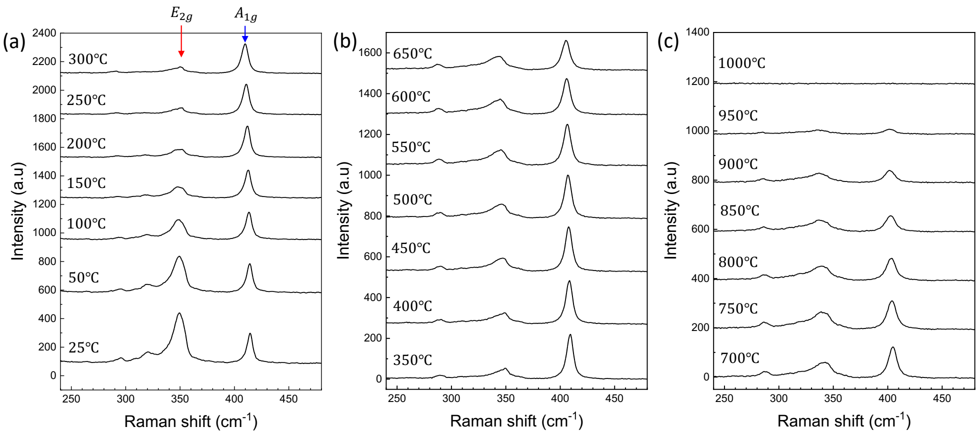


Figure S1: Temperature-dependent Raman spectra of monolayer $WS_2$ measured in vacuum. (a) Raman spectra recorded from 25 °C to 300 °C. (b) Raman spectra recorded from 350 °C to 650 °C. (c) Raman spectra recorded from 700 °C to 1000 °C.

In addition to the intensity reduction, both Raman peak positions exhibit a redshift with increasing temperature. Figure S2 displays the temperature dependence of the $A_{1g}$ mode's shift in Both Stokes and Anti-Stokes (in absolute value). A linear behavior is observed, with a slope of $-0.0134$ cm$^{-1}$/°C. This value is comparable to previously reported results, where a linear fit of the Raman shift was obtained in the temperature range from 100 K to 600 K with a slope of approximately $-0.0121$ cm$^{-1}$/K [1]. The close agreement in slope confirms the consistency of our measurements, while the extended temperature range investigated here allows for a clearer assessment of the linear temperature dependence of the $A_{1g}$ mode.

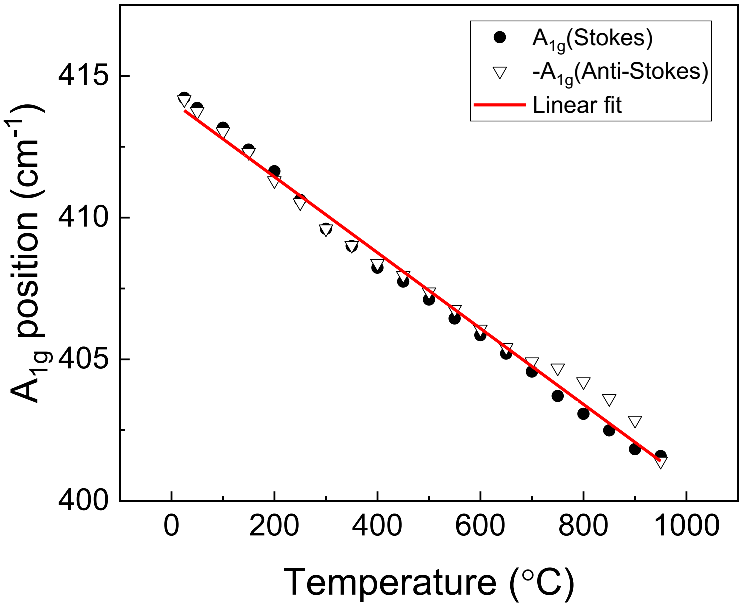


Figure S2: Temperature dependence of the $A_{1g}$ Raman mode position in both Stokes and anti-Stokes, showing a linear redshift with increasing temperature.

Figure S3(a) shows an optical image of the sample used for the Raman measurements mentioned above. The maximum annealing temperature was 1200°C, after which the flake was no longer visible in the microscope image S3(b). The absence of Raman features above 1000° C suggest that around this temperature the sample undergoes thermal dissociation.

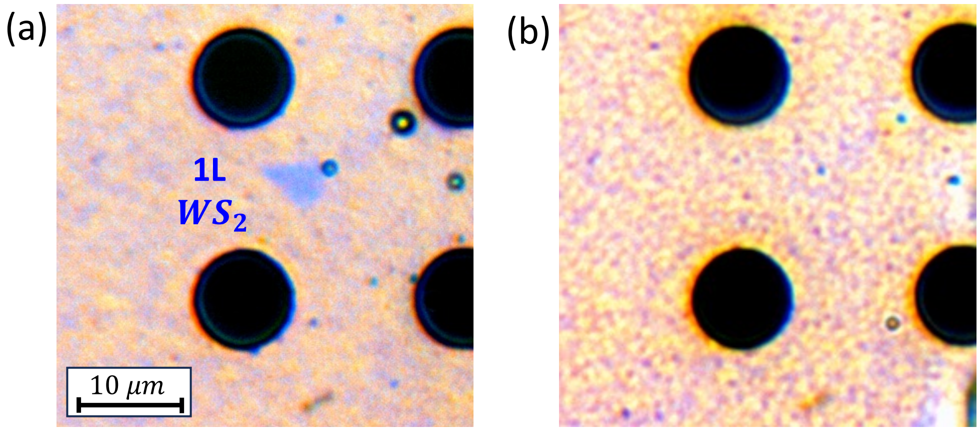


Figure S3: Optical image of a non-encapsulated sample on the membrane (a) before annealing, (b) after annealing up to 1200 °C.

## Lateral displacement of the membrane during annealing

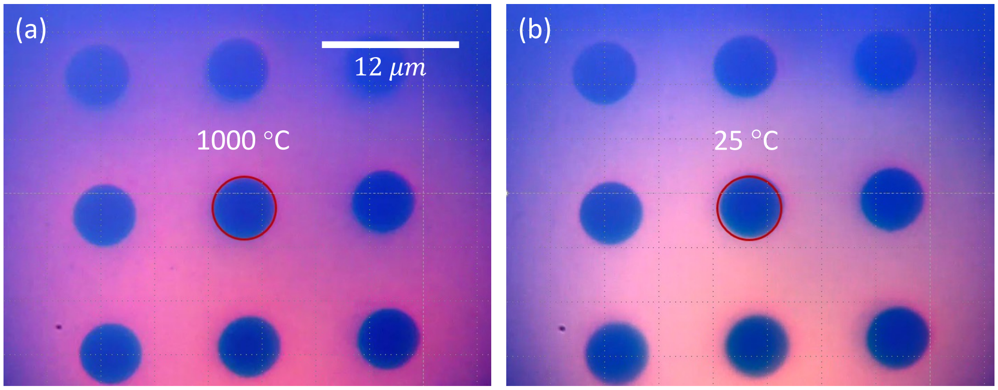


Figure S4: Optical image under white light illumination of SiC membrane at (a) 1000°C and (b) at 25°.

Figure S4 (a) shows an optical image under white light illumination of one of the SiC membranes at 1000 °C. The red circle indicates the initial position of the central hole of the membrane on the imaging camera. After cooling down back to room temperature, the obtained image (Fig. S4 (b)) shows negligible (sub $\mu$m) lateral shift. This remarkable stability allows to study the optical signatures of the same fixed spot on the sample after being subjected to different annealing cycles. The difference in apparent color between both images is due to the presence of visible blackbody radiation at 1000 °C.

## Extended temperature calibration using blackbody radiation

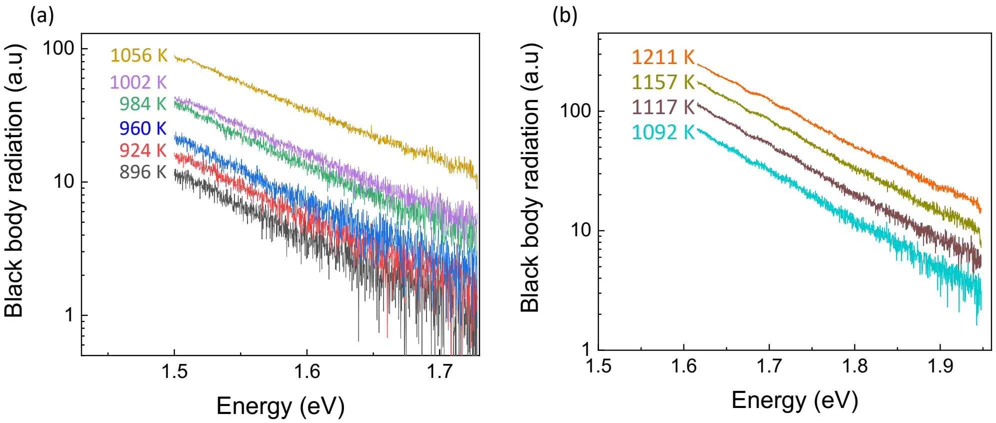


Figure S5: Blackbody radiation spectra of the suspended membrane used for extended temperature calibration at high temperatures. The spectra are fitted using Planck's law. (a)From 896 K to 1056 K, (b) from 1092 K to 1211 K

As discussed in the main text, the temperature of the sample can be calibrated using the neutral exciton energy position from cryogenic temperatures up to 925 K. Figure S5 presents the blackbody radiation emitted by the membrane, which provides an extended temperature calibration at elevated temperatures. The blackbody spectra are fitted, after being corrected by the spectral response of the setup, using Planck's law:

$$B(\nu, T) = A(h\nu)^2 \frac{1}{e^{h\nu/kT} - 1}.$$

At 925 K (determined from the exciton position), the temperature estimated from the blackbody radiation fit yields 924±3.4 K, in excellent agreement with the exciton-based calibration obtained from Passler's model. More generally, the discrepancy between the two calibration methods remains within only a few kelvin.

## Other defect-related emission in $WS_2$

The evolution of the PL spectra under thermal annealing was investigated in more than 5 encapsulated different samples. Several of them showed the emergence of narrow emission after 800K annealing. This line becomes spectrally isolated after annealing at 900 K, as shown in Figure S6 (a) and (b). This emission line $X'_L$ is approximately 120 meV below the neutral exciton $X_A^0$. As shown in Figure S6 (c), the emission intensity initially increases with excitation power and saturates above approximately 6 $\mu$W, which is a characteristic signature of emission from a finite density of localized defect states.

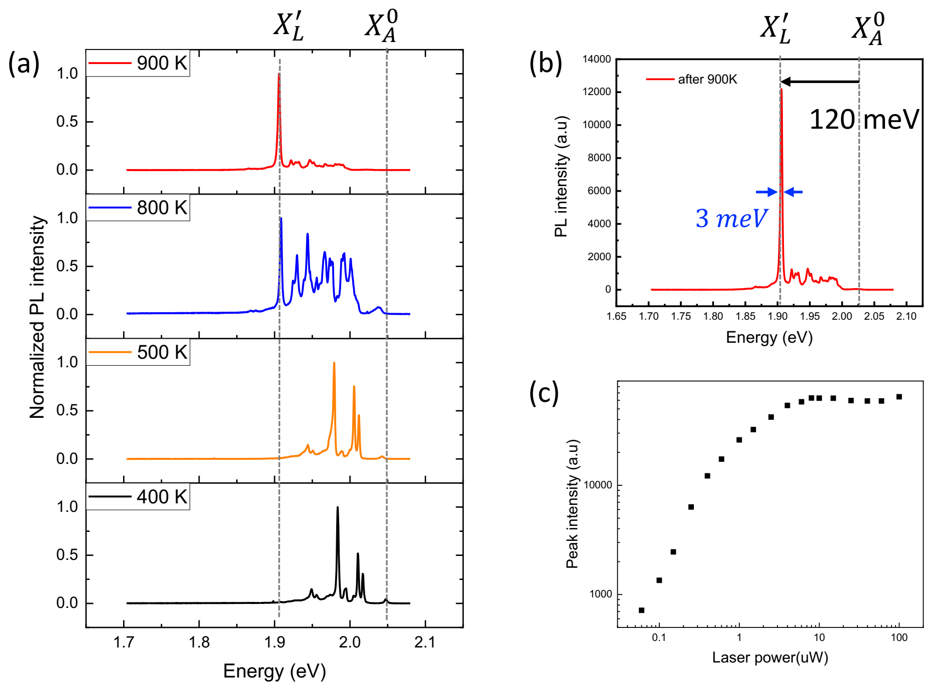


Figure S6: (a) Low-temperature PL spectra of an hBN-encapsulated WS2 monolayer measured at $T = 3.6$ K after annealing at 400, 500, 800, and 900 K for 30 min. ($\lambda_{laser} = 514.5$ nm (CW), $P_{\text{laser}} = 1$ $\mu$W.) (b) PL spectrum recorded after annealing at 900 K, showing the emergence of a new narrow emission peak $X_L$ located approximately 120 meV below the neutral exciton $X_A^0$. (c) Power-dependent PL intensity of the $X_L$ peak.

We also performed annealing experiments on non-encapsulated monolayers. Figure S7 summarizes the results of these experiments on one of the samples. As shown in Figure S7(a), the clear emergence of a new emission peak in the PL spectra is observed starting from an annealing temperature of 1000 K. With increasing annealing temperature, the emission peak becomes progressively narrower. Figure S7(b) displays the narrowest emission peak obtained when scanning the sample, with a measured linewidth of 12 meV. In addition, power-dependent measurements again reveal a clear saturation behavior of the emission intensity, characteristic of defect-related emission (Figure S7 (c)). The peak is located approximately 220 meV below the neutral exciton energy. The increased energy separation with respect to the encapsulated samples may be attributed to the well-known reduction of exciton binding energy, typically by about a factor of two. Considering this reduction factor, we think that it is likely that this emission is of the same nature as the $X'_L$ one observed in encapsulated samples.

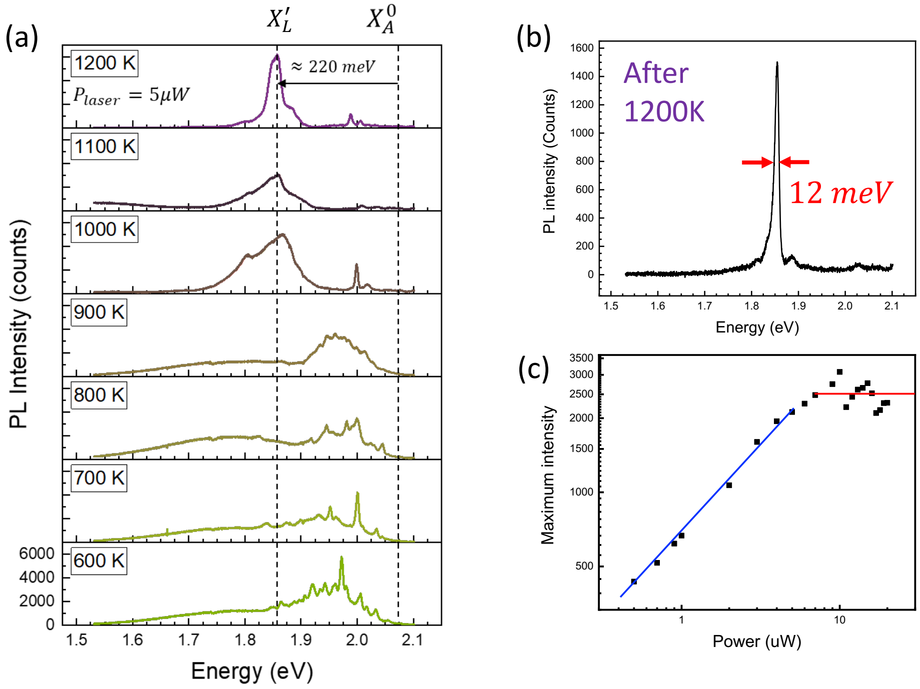


Figure S7: (a) Low-temperature ($T = 30$ K) PL spectra of non-encapsulated $WS_2$ monolayer measured after annealing at different temperatures . (b) Narrowest peak $X'_L$ in the PL spectrum obtained after annealing at 1200 K. (c) Power-dependent PL intensity of the XL peak measured using a CW laser ($\lambda_{\text{laser}} = 570$ nm).

## Power-dependence measurements

In this section, we provide details on the modeling of the saturation behavior observed in the power-dependent measurements shown in Figure 3(b). In the saturation regime, only one photon per laser pulse can be emitted, as the emitter lifetime (0.9 ns) is much longer than the laser pulse duration (40 ps), and much shorter than the interval between laser pulses (12.8 ns). Therefore, the PL intensity is simply given by the product of the laser repetition rate $f_{rep}$, the quantum yield $\Phi_y$, and the optical collection efficiency $\eta_{opt}$ of the setup.

$$I_{PL}\,(\mathrm{s}^{-1}) = f_{rep}\,\Phi_y\,\eta_{opt}, \qquad \text{(saturation regime)}$$

Outside the saturation regime, the probability that the emitter is excited during a laser pulse ($P_{exc}$) must be considered. The PL intensity can then be generally written as

$$I_{PL}\,(\mathrm{s}^{-1}) = P_{exc}\,f_{rep}\,\Phi_y\,\eta_{opt}.$$

If $P_\gamma$ denotes the probability that a single photon excites the emitter, the excitation probability can be expressed as

$$P_{exc} = 1 - (1 - P_\gamma)^{N_\gamma},$$

where $N_\gamma$ is the number of laser photons per laser pulse. This can be approximated, if $P_\gamma / N_\gamma \ll 1$, as

$$P_{exc} \simeq 1 - e^{-N_\gamma P_\gamma}$$

Therefore, the power-dependent PL intensity can be fitted using the exponential form

$$I_{PL}(P_{avg}) \propto 1 - e^{-\frac{a}{f_{rep}} P_{avg}}.$$

By comparing the two expressions above, we obtain $P_\gamma = \alpha h\nu$. From the exponential fit shown in Figure3(b), $\alpha = 6.92 \times 10^{12}\ \mathrm{J}^{-1}$, which yields $P_\gamma = 2.73 \times 10^{-6}$ when multiplied by the photon energy $h\nu$.

The quantum yield $\Phi_y$ can be directly extracted in the saturation regime as

$$QY = \frac{R_{APD1} + R_{APD2}}{f_{rep}\, \eta_{opt}},$$

where $R_{APD1}$ and $R_{APD2}$ are the photon count rates detected by the two single-photon avalanche diodes (SPADs). Using a total detected count rate of 1000 counts/s and an optical collection efficiency of $\eta_{opt} = 2.44 \times 10^{-4}$—which accounts for losses in the objective, mirrors, beam splitter, filters, and coupling from the spectrometer to the SPADs—the resulting quantum yield is estimated to be $\sim 5.25\%$.

# References


(1) Huang, X.; Gao, Y.; Yang, T.; Ren, W.; Cheng, H.-M.; Lai, T. Quantitative Analysis of Temperature Dependence of Raman Shift of Monolayer WS2. *Scientific Reports* **2016**, *6*, 32236.
